# Supplementary material for: SimCADO - an instrument data simulator package for MICADO at the E-ELT
Source: arXiv:1609.01480 source file (2016-09-06)
Supplement: Supplementary file 1 [file 8_appendix.tex]

\section{Using external PSF kernels in SimCADO}

Description of how to use FITS files for SimCADO

\begin{table}[h]
    \centering
    \begin{tabular}{| p{0.15\textwidth} | p{0.07\textwidth} | p{0.7\textwidth} |}
        \hline
        Header Keyword  & Units & Description \\
        \hline
        NAXIS1 & pixels & The side length in the image. It is assumed that the PSF kernel is square \\
        CDELT1 & arcsec & The pixel scale of the FITS image in this extension \\
        WAVELENG & \textmu m & The PSF kernel corresponds to this wavelength \\
        \hline
    \end{tabular}
    \caption{Keywords needed in the header of a FITS file containing a PSF kernel}
    \label{tab:psf_header_keys}
\end{table}
